# Supplementary material for: Realizing Reduced and Sparse Biochemical Reaction Networks from Dynamics
Source: arXiv:2508.18096 ancillary file (2025-08-26)
Supplement: Supplementary file 1 [file supplementary.pdf]

# Realizing Reduced and Sparse Biochemical Reaction Networks from Dynamics Supplementary Material

Maurice Filo and Mustafa Khammash

## Appendix

### A. Numerical Values of Estimated Parameters

The values of $\boldsymbol{\theta}$ for Figs. 1(b) and 2(b) respectively are

$$\begin{array}{c} \begin{matrix} 1 & x_1 & x_2 & x_1^2 & x_1x_2 & x_2^2 \end{matrix} \\ \begin{bmatrix} 0.2961 & -0.1295 & 0 & 0.6811 & -0.6328 & 0 \\ 0.4181 & 0.0372 & -0.5114 & 0.3707 & -0.2328 & 0.0765 \end{bmatrix} \begin{matrix} \dot{x}_1 \\ \dot{x}_2 \end{matrix} \end{array}$$

$$\begin{array}{c} \begin{matrix} 1 & x_1 & x_2 & x_3 & x_1^2 & x_1x_2 & x_1x_3 & x_2^2 & x_2x_3 & x_3^2 \end{matrix} \\ \begin{bmatrix} 2.8629 & -0.1074 & 0.0076 & 0.1516 & 0.5918 & -3.7640 & -1.0898 & 0.0002 & 0.0001 & 0 \\ 0.0058 & 0.0936 & -4.1926 & 0.0003 & 1.2222 & -5.9597 & 0.0037 & -0.4057 & 1.2474 & 1.5000 \\ 0.0000 & 0.0001 & 0.0000 & -2.1880 & 0.0108 & 0.0261 & 3.8425 & 0.0004 & -6.8494 & 2.7221 \end{bmatrix} \begin{matrix} \dot{x}_1 \\ \dot{x}_2 \\ \dot{x}_3 \end{matrix} \end{array}$$

### B. Calculation of the Proximal Operator

From the definition of $\text{prox}_{h,\alpha}(\boldsymbol{\theta})$ given in Equation (11) of the main text, we have

$$\begin{aligned} \text{prox}_{h,\alpha}(\boldsymbol{\theta}) &= \underset{\tilde{\boldsymbol{\theta}}}{\text{argmin}} \ \frac{1}{2\alpha}\|\boldsymbol{\theta} - \tilde{\boldsymbol{\theta}}\|_F^2 + \lambda\|\tilde{\boldsymbol{\theta}}\|_1 + \mathcal{I}_+(S \circ \tilde{\boldsymbol{\theta}}) \\ &= \underset{S\circ\tilde{\boldsymbol{\theta}}\geq 0}{\text{argmin}} \ \frac{1}{2\alpha}\|\boldsymbol{\theta} - \tilde{\boldsymbol{\theta}}\|_F^2 + \lambda\|\tilde{\boldsymbol{\theta}}\|_1 \\ &= \underset{S\circ\tilde{\boldsymbol{\theta}}\geq 0}{\text{argmin}} \ \frac{1}{2\alpha}\sum_{i,j=1}^{n,m}\left(\theta_{ij} - \tilde{\theta}_{ij}\right)^2 + \lambda\sum_{i,j=1}^{n,m}|\tilde{\theta}_{ij}|. \end{aligned}$$

Now, let $S \in \{0,1\}^{n\times m}$ be a binary selector matrix whose entries are zero everywhere except at positions $(i,j) \in \mathcal{J}^+$, where they are set to one. These selected entries enforce the constraint that $\theta_{ij} \geq 0$ for all $(i,j) \in \mathcal{J}^+$. Hence, we have

$$\begin{aligned} \hat{\boldsymbol{\theta}} &\triangleq \text{prox}_{h,\alpha}(\boldsymbol{\theta}) \\ &= \underset{\tilde{\theta}_{ij}\geq 0, \forall (i,j)\in\mathcal{J}^+}{\text{argmin}} \ \frac{1}{2\alpha}\sum_{i,j}\left(\theta_{ij} - \tilde{\theta}_{ij}\right)^2 \\ &\qquad + \lambda\sum_{(i,j)\in\mathcal{J}^+}\tilde{\theta}_{ij} + \lambda\sum_{(i,j)\notin\mathcal{J}^+}|\tilde{\theta}_{ij}|. \end{aligned}$$

Since the terms of the sums are independent, one can minimize each summation term separately, that is

$$\text{For } (i,j) \in \mathcal{J}^+: \quad \hat{\theta}_{ij} = \underset{\tilde{\theta}_{ij}\geq 0}{\text{argmin}} \ \frac{1}{2\alpha}\left(\theta_{ij} - \tilde{\theta}_{ij}\right)^2 + \lambda\tilde{\theta}_{ij}$$

$$\text{For } (i,j) \notin \mathcal{J}^+: \quad \hat{\theta}_{ij} = \text{argmin} \ \frac{1}{2\alpha}\left(\theta_{ij} - \tilde{\theta}_{ij}\right)^2 + \lambda|\tilde{\theta}_{ij}|.$$

For $(i,j) \in \mathcal{J}^+$, the minimization is achieved for $\hat{\theta}_{ij} = \theta_{ij} - \lambda\alpha$ when $\theta_{ij} > \lambda\alpha$, and for $\hat{\theta}_{ij} = 0$ otherwise. For $(i,j) \notin \mathcal{J}^+$, the minimization is achieved for $\hat{\theta}_{ij} = \theta_{ij} - \lambda\alpha$ when $\theta_{ij} > \lambda\alpha$, $\hat{\theta}_{ij} = \theta_{ij} + \lambda\alpha$ when $\theta_{ij} < -\lambda\alpha$ and for $\hat{\theta}_{ij} = 0$ otherwise. This can be compactly written as follows

$$\text{For } (i,j) \in \mathcal{J}^+: \quad \hat{\theta}_{ij} = \max\left\{\theta_{ij} - \lambda\alpha, 0\right\}$$

$$\text{For } (i,j) \notin \mathcal{J}^+: \quad \hat{\theta}_{ij} = \text{sign}(\theta_{ij})\max\left\{|\theta_{ij}| - \lambda\alpha, 0\right\}.$$

By exploiting the fact that $|\theta_{ij}| = \text{sign}(\theta_{ij})\,\theta_{ij}$, one can rewrite the result in a more compact matrix form as

$$\hat{\boldsymbol{\theta}} = \max\left\{S\circ\boldsymbol{\theta} - \lambda\alpha, 0\right\} + \text{sign}\left(\bar{S}\circ\boldsymbol{\theta}\right)\circ\max\left\{|\bar{S}\circ\boldsymbol{\theta}| - \lambda\alpha, 0\right\}.$$

### C. Calculation of the Gradient

Let $\langle.,.\rangle_{\mathbb{L}_n^2[0,T]}$ (resp. $\langle.,.\rangle_{\mathbb{R}^{n\times m}}$) denote the inner product in $\mathbb{L}_n^2[0,T]$ (resp. $\mathbb{R}^{n\times m}$). Hence, if $x, y \in \mathbb{L}_n^2[0,T]$ and $A, B \in \mathbb{R}^{n\times m}$ then

$$\begin{aligned} \langle x, y\rangle_{\mathbb{L}_n^2[0,T]} &\triangleq \int_0^T x^T(t)y(t)dt \\ \langle A, B\rangle_{\mathbb{R}^{n\times m}} &\triangleq \text{tr}\left(A^TB\right). \end{aligned}$$

Furthermore, let $\|.\|^2_{\mathbb{L}_n^2[0,T]} \triangleq \langle.,.\rangle_{\mathbb{L}_n^2[0,T]}$ denote the associated norm squared in $\mathbb{L}_n^2[0,T]$. Let's calculate the directional derivative of $J$, in the direction of $\tilde{\boldsymbol{\theta}}$, evaluated at $\bar{\boldsymbol{\theta}}$.

$$\begin{aligned} \partial J_{\bar{\boldsymbol{\theta}}}(\tilde{\boldsymbol{\theta}}) &\triangleq \lim_{\epsilon\to 0}\frac{1}{\epsilon}\left\{J(\bar{\boldsymbol{\theta}} + \epsilon\tilde{\boldsymbol{\theta}}) - J(\bar{\boldsymbol{\theta}})\right\} \\ &= \lim_{\epsilon\to 0}\frac{1}{2\epsilon}\Big\{\|\mathcal{M}(\bar{\boldsymbol{\theta}} + \epsilon\tilde{\boldsymbol{\theta}}) - y_T\|^2_{\mathbb{L}_q^2[0,T]} \\ &\qquad\qquad - \|\mathcal{M}(\bar{\boldsymbol{\theta}}) - y_T\|^2_{\mathbb{L}_q^2[0,T]}\Big\} \\ &= \lim_{\epsilon\to 0}\frac{1}{2\epsilon}\Big\{\|\mathcal{M}(\bar{\boldsymbol{\theta}}) + \epsilon\partial\mathcal{M}_{\bar{\boldsymbol{\theta}}}(\tilde{\boldsymbol{\theta}}) - y_T\|^2_{\mathbb{L}_q^2[0,T]} \\ &\qquad\qquad - \|\mathcal{M}(\bar{\boldsymbol{\theta}}) - y_T\|^2_{\mathbb{L}_q^2[0,T]}\Big\} \\ &= \left\langle\mathcal{M}(\bar{\boldsymbol{\theta}}) - y_T, \partial\mathcal{M}_{\bar{\boldsymbol{\theta}}}(\tilde{\boldsymbol{\theta}})\right\rangle_{\mathbb{L}_q^2[0,T]} \\ &= \left\langle\partial\mathcal{M}^*_{\bar{\boldsymbol{\theta}}}\left(\mathcal{M}(\bar{\boldsymbol{\theta}}) - y_T\right), \tilde{\boldsymbol{\theta}}\right\rangle_{\mathbb{R}^{n\times m}} \triangleq \left\langle\nabla J_{\bar{\boldsymbol{\theta}}}, \tilde{\boldsymbol{\theta}}\right\rangle_{\mathbb{R}^{n\times m}}, \end{aligned}$$

where $\partial\mathcal{M}_{\bar{\boldsymbol{\theta}}}$ and $\partial\mathcal{M}^*_{\bar{\boldsymbol{\theta}}}$ are the directional derivatives of $\mathcal{M}$ and its adjoint, evaluated at $\bar{\boldsymbol{\theta}}$. That is, the gradient of $J$, evaluated at $\bar{\boldsymbol{\theta}}$ is given by $\nabla J_{\bar{\boldsymbol{\theta}}} = \partial\mathcal{M}^*_{\bar{\boldsymbol{\theta}}}\left(\mathcal{M}(\bar{\boldsymbol{\theta}}) - y_T\right)$. We now calculate the linear operators $\partial\mathcal{M}_{\bar{\boldsymbol{\theta}}}$ and $\partial\mathcal{M}^*_{\bar{\boldsymbol{\theta}}}$.

**Directional Derivative Operator $\partial\mathcal{M}_{\bar{\boldsymbol{\theta}}}$.** Define the parameter-to-state operator $\mathcal{S}: \mathbb{R}^{n\times m} \to \mathbb{L}_n^2[0,T]$ as

$$x = \mathcal{S}(\boldsymbol{\theta}) \iff \dot{x} = \boldsymbol{\theta}\Phi(x), \qquad x(0) = x_0. \tag{1}$$

The corresponding parameter-to-output operator is then given by $\mathcal{M} = C\mathcal{S}$, and the action of its directional derivative evaluated at $\bar{\boldsymbol{\theta}}$ on $\tilde{\boldsymbol{\theta}}$ is

$$\partial\mathcal{M}_{\bar{\boldsymbol{\theta}}}(\tilde{\boldsymbol{\theta}}) = C\left(\partial\mathcal{S}_{\bar{\boldsymbol{\theta}}}(\tilde{\boldsymbol{\theta}})\right), \tag{2}$$

where $\partial\mathcal{S}_{\bar{\boldsymbol{\theta}}}$ denotes the directional derivative of $\mathcal{S}$ evaluated at $\bar{\boldsymbol{\theta}}$. To compute $\partial\mathcal{S}_{\bar{\boldsymbol{\theta}}}$, we perform a first-order perturbation analysis around $\bar{\boldsymbol{\theta}}$. Perturbing $\bar{\boldsymbol{\theta}}$ by $\epsilon\tilde{\boldsymbol{\theta}}$, we expand $\mathcal{S}(\bar{\boldsymbol{\theta}} + \epsilon\tilde{\boldsymbol{\theta}})$ via a Taylor series:

$$\mathcal{S}(\bar{\boldsymbol{\theta}} + \epsilon\tilde{\boldsymbol{\theta}}) = \mathcal{S}(\bar{\boldsymbol{\theta}}) + \epsilon\partial\mathcal{S}_{\bar{\boldsymbol{\theta}}}(\tilde{\boldsymbol{\theta}}) + \mathcal{O}(\epsilon^2). \tag{3}$$

Define the following variables:

$$x_\epsilon \triangleq \mathcal{S}(\bar{\boldsymbol{\theta}} + \epsilon\tilde{\boldsymbol{\theta}}), \quad \bar{x} \triangleq \mathcal{S}(\bar{\boldsymbol{\theta}}), \quad \tilde{x} \triangleq \partial\mathcal{S}_{\bar{\boldsymbol{\theta}}}(\tilde{\boldsymbol{\theta}}), \tag{4}$$

so that (3) becomes

$$x_\epsilon = \bar{x} + \epsilon\tilde{x} + \mathcal{O}(\epsilon^2). \tag{5}$$

From the definition of $\mathcal{S}$ in (1), the perturbed trajectory $x_\epsilon$ satisfies

$$x_\epsilon = \mathcal{S}(\bar{\boldsymbol{\theta}}+\epsilon\tilde{\boldsymbol{\theta}}) \iff \dot{x}_\epsilon = (\bar{\boldsymbol{\theta}} + \epsilon\tilde{\boldsymbol{\theta}})\Phi(x_\epsilon), \qquad x_\epsilon(0) = x_0. \tag{6}$$

Substituting (5) into (6) and retaining terms up to first order in $\epsilon$, we obtain:

$$\dot{\bar{x}} + \epsilon\dot{\tilde{x}} = (\bar{\boldsymbol{\theta}} + \epsilon\tilde{\boldsymbol{\theta}})\Phi(\bar{x} + \epsilon\tilde{x}), \qquad \bar{x}(0) + \epsilon\tilde{x}(0) = x_0.$$

From the initial condition, we match powers of $\epsilon$ to get $\bar{x}(0) = x_0$ and $\tilde{x}(0) = 0$. As for the differential equation, expanding $\Phi(\bar{x} + \epsilon\tilde{x})$ via Taylor series around $\bar{x}$ yields

$$\dot{\bar{x}} + \epsilon\dot{\tilde{x}} = \bar{\boldsymbol{\theta}}\Phi(\bar{x}) + \epsilon\left(\bar{\boldsymbol{\theta}}\,\partial\Phi_{\bar{x}}\tilde{x} + \tilde{\boldsymbol{\theta}}\Phi(\bar{x})\right).$$

Matching terms of equal order in $\epsilon$, we conclude:

$$\tilde{x} = \partial\mathcal{S}_{\bar{\boldsymbol{\theta}}}(\tilde{\boldsymbol{\theta}}) \iff \dot{\tilde{x}} = \bar{\boldsymbol{\theta}}\,\partial\Phi_{\bar{x}}\tilde{x} + \tilde{\boldsymbol{\theta}}\Phi(\bar{x}), \qquad \tilde{x}(0) = 0, \tag{7}$$

where $\bar{x} = \mathcal{S}(\bar{\boldsymbol{\theta}})$. Substituting this result into (2) yields the directional derivative of the parameter-to-output map $\partial\mathcal{M}_{\bar{\boldsymbol{\theta}}}$, as summarized in the second row of Table I.

**Adjoint Operator $\partial\mathcal{M}^*_{\bar{\boldsymbol{\theta}}}$.** Define the time derivative operator $\mathcal{D}_0$, which maps a differentiable signal $x$ with zero initial condition to its time derivative, i.e. $\mathcal{D}_0 x = \dot{x}$, with $x(0) = 0$. Using this notation, we can express the action of $\partial\mathcal{M}_{\bar{\boldsymbol{\theta}}}$ on a perturbation $\tilde{\boldsymbol{\theta}}$ in terms of $\mathcal{D}_0$, starting from the second row of Table I. Specifically:

$$\tilde{y} = \partial\mathcal{M}_{\bar{\boldsymbol{\theta}}}(\tilde{\boldsymbol{\theta}}) \iff \begin{cases} \left(\mathcal{D}_0 - \bar{\boldsymbol{\theta}}\,\partial\Phi(\bar{x})\right)\tilde{x} = \tilde{\boldsymbol{\theta}}\,\Phi(\bar{x}) \\ \tilde{y} = C\tilde{x} \end{cases}$$
$$\iff \tilde{y} = C\left(\mathcal{D}_0 - \bar{\boldsymbol{\theta}}\,\partial\Phi(\bar{x})\right)^{-1}\tilde{\boldsymbol{\theta}}\,\Phi(\bar{x}). \tag{8}$$

It is straightforward to show that the adjoint of $\mathcal{D}_0$ is $-\mathcal{D}_T$, where $\mathcal{D}_T$ is another time derivative operator, but defined on functions with zero terminal condition, i.e. $\mathcal{D}_T x = \dot{x}$, with $x(T) = 0$. The duality $\mathcal{D}_0^* = -\mathcal{D}_T$, combined with the abstract representation of $\partial\mathcal{M}_{\bar{\boldsymbol{\theta}}}$ in (8), allows us to easily calculate the adjoint $\partial\mathcal{M}^*_{\bar{\boldsymbol{\theta}}}$ as follows. Let $\hat{y} \in \mathbb{L}^2_q[0,T]$ and $\tilde{\boldsymbol{\theta}} \in \mathbb{R}^{n\times m}$. Then,

$$\begin{aligned}
&\langle \hat{y}, \partial\mathcal{M}_{\bar{\boldsymbol{\theta}}}(\tilde{\boldsymbol{\theta}})\rangle_{\mathbb{L}^2_q[0,T]} \\
&\quad= \left\langle \hat{y}, C\left(\mathcal{D}_0 - \bar{\boldsymbol{\theta}}\,\partial\Phi(\bar{x})\right)^{-1}\tilde{\boldsymbol{\theta}}\,\Phi(\bar{x})\right\rangle_{\mathbb{L}^2_q[0,T]} \\
&\quad= \left\langle \left(\mathcal{D}_0 - \bar{\boldsymbol{\theta}}\,\partial\Phi(\bar{x})\right)^{-*}C^T\hat{y}, \tilde{\boldsymbol{\theta}}\,\Phi(\bar{x})\right\rangle_{\mathbb{L}^2_q[0,T]} \\
&\quad= \left\langle -\left(\mathcal{D}_T + \partial\Phi(\bar{x})^T\bar{\boldsymbol{\theta}}^T\right)^{-1}C^T\hat{y}, \tilde{\boldsymbol{\theta}}\,\Phi(\bar{x})\right\rangle_{\mathbb{L}^2_q[0,T]},
\end{aligned}$$

where the first equality follows from (8), the second uses the adjoint of $\left(\mathcal{D}_0 - \bar{\boldsymbol{\theta}}\,\partial\Phi(\bar{x})\right)^{-1}$ to move it to the other side of the inner product, and the third follows from $\mathcal{D}_0^* = -\mathcal{D}_T$. Define the intermediate signal

$$\bar{\lambda} \triangleq -\left(\mathcal{D}_T + \partial\Phi(\bar{x})^T\bar{\boldsymbol{\theta}}^T\right)^{-1}C^T\hat{y}. \tag{9}$$

Then, we proceed as follows

$$\begin{aligned}
\langle \hat{y}, \partial\mathcal{M}_{\bar{\boldsymbol{\theta}}}(\tilde{\boldsymbol{\theta}})\rangle_{\mathbb{L}^2_q[0,T]} &= \int_0^T \bar{\lambda}^T(t)\tilde{\boldsymbol{\theta}}\,\Phi[\bar{x}(t)]dt \\
&= \int_0^T \mathrm{tr}\left(\bar{\lambda}^T(t)\tilde{\boldsymbol{\theta}}\,\Phi[\bar{x}(t)]\right)dt \\
&= \int_0^T \mathrm{tr}\left(\Phi[\bar{x}(t)]\bar{\lambda}^T(t)\tilde{\boldsymbol{\theta}}\right)dt \\
&= \mathrm{tr}\left(\int_0^T \Phi[\bar{x}(t)]\bar{\lambda}^T(t)dt\;\tilde{\boldsymbol{\theta}}\right) \\
&= \left\langle \int_0^T \bar{\lambda}(t)\Phi^T[\bar{x}(t)]dt, \tilde{\boldsymbol{\theta}}\right\rangle_{\mathbb{R}^{n\times m}} \\
&\triangleq \langle \mathcal{M}^*_{\bar{\boldsymbol{\theta}}}(\hat{y}), \tilde{\boldsymbol{\theta}}\rangle_{\mathbb{R}^{n\times m}}.
\end{aligned}$$

Therefore, the adjoint operator is given by

$$\partial\mathcal{M}^*_{\bar{\boldsymbol{\theta}}}(\hat{y}) = \int_0^T \bar{\lambda}(t)\,\Phi^T[\bar{x}(t)]\,dt,$$

where $\bar{\lambda}$ is defined in (9). This result is summarized in the third row of Table I. Finally, the gradient can be calculated as follows

$$\nabla J_{\bar{\boldsymbol{\theta}}} = \partial\mathcal{M}^*_{\bar{\boldsymbol{\theta}}}\left(\mathcal{M}(\bar{\boldsymbol{\theta}}) - y_T\right) = \int_0^T \bar{\lambda}(t)\Phi^T\left[\bar{x}(t)\right]dt, \text{ with}$$
$$\begin{cases} \dot{\bar{x}} = \bar{\boldsymbol{\theta}}\Phi(\bar{x}); & \bar{x}(0) = x_0 \\ \bar{y} = C\bar{x} & \\ \dot{\bar{\lambda}} = -\left[\bar{\boldsymbol{\theta}}\partial\Phi(\bar{x})\right]^T\bar{\lambda} - C^T(\bar{y} - y_T); & \bar{\lambda}(T) = 0. \end{cases}$$

| Operator | Differential Equations |
|---|---|
| $\mathcal{M} : \mathbb{R}^{n\times m} \to \mathbb{L}_q^2[0,T]$ | $\bar{y} = \mathcal{M}(\bar{\boldsymbol{\theta}}) \quad \Longleftrightarrow \quad \begin{cases} \dot{\bar{x}} = \bar{\boldsymbol{\theta}}\Phi(\bar{x}); \quad \bar{x}(0) = x_0 \\ \bar{y} = C\bar{x} \end{cases}$ |
| $\partial\mathcal{M}_{\bar{\boldsymbol{\theta}}} : \mathbb{R}^{n\times m} \to \mathbb{L}_q^2[0,T]$ | $\tilde{y} = \partial\mathcal{M}_{\bar{\boldsymbol{\theta}}}(\tilde{\boldsymbol{\theta}}) \quad \Longleftrightarrow \quad \begin{cases} \dot{\tilde{x}} = \bar{\boldsymbol{\theta}}\partial\Phi(\bar{x})\tilde{x} + \tilde{\boldsymbol{\theta}}\Phi(\bar{x}); \quad \tilde{x}(0) = 0 \\ \tilde{y} = C\tilde{x} \end{cases}$ |
| $\partial\mathcal{M}^*_{\bar{\boldsymbol{\theta}}} : \mathbb{L}_q^2[0,T] \to \mathbb{R}^{n\times m}$ | $\hat{\boldsymbol{\theta}} = \partial\mathcal{M}^*_{\bar{\boldsymbol{\theta}}}(\hat{y}) \quad \Longleftrightarrow \quad \begin{cases} \hat{\boldsymbol{\theta}} = \int_0^T \bar{\lambda}(t)\Phi^T[\bar{x}(t)]dt \\ \dot{\bar{\lambda}} = -\left[\bar{\boldsymbol{\theta}}\partial\Phi(\bar{x})\right]^T\bar{\lambda} - C^T\hat{y}; \quad \bar{\lambda}(T) = 0 \end{cases}$ |

**TABLE I**: The Parameter-to-Output Operator $\mathcal{M}$
